# Supplementary material for: Identity Overlap Between Face Recognition Train/Test Data: Causing Optimistic Bias in Accuracy Measurement
Source: arXiv:2405.09403 source file (2024-05-15)
Supplement: Supplementary file 1 [file same_identity.tex]

\begin{figure*}[t]
    \centering
    \captionsetup[subfigure]{labelformat=empty}
    \begin{subfigure}[b]{0.9\linewidth}
        \begin{subfigure}[b]{1\linewidth}
            \begin{subfigure}[b]{0.24\linewidth}
                \includegraphics[width=\linewidth]{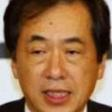}
                \caption{Naoto\_Kan\_2}
            \end{subfigure}
            \begin{subfigure}[b]{0.24\linewidth}
                \includegraphics[width=\linewidth]{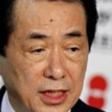}
                \caption{0\_5858920/82}
            \end{subfigure}
            \begin{subfigure}[b]{0.24\linewidth}
                \includegraphics[width=\linewidth]{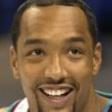}
                \caption{Drew\_Gooden\_1}
            \end{subfigure}
            \begin{subfigure}[b]{0.24\linewidth}
                \includegraphics[width=\linewidth]{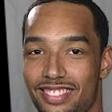}
                \caption{0\_5870377/25}
            \end{subfigure}
        \end{subfigure}
        \begin{subfigure}[b]{1\linewidth}
            \begin{subfigure}[b]{0.24\linewidth}
                \includegraphics[width=\linewidth]{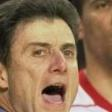}
                \caption{Rick\_Pitino\_4}
            \end{subfigure}
            \begin{subfigure}[b]{0.24\linewidth}
                \includegraphics[width=\linewidth]{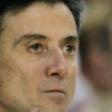}
                \caption{0\_5859710/40}
            \end{subfigure}
            \begin{subfigure}[b]{0.24\linewidth}
                \includegraphics[width=\linewidth]{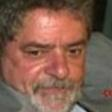}
                \caption{Luiz\_Inacio\_Lula\_da\_Silva\_2}
            \end{subfigure}
            \begin{subfigure}[b]{0.24\linewidth}
                \includegraphics[width=\linewidth]{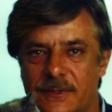}
                \caption{0\_5835410/64}
            \end{subfigure}
        \end{subfigure}

        \begin{subfigure}[b]{1\linewidth}
            \begin{subfigure}[b]{0.24\linewidth}
                \includegraphics[width=\linewidth]{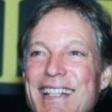}
                \caption{Richard\_Chamberlain\_1}
            \end{subfigure}
            \begin{subfigure}[b]{0.24\linewidth}
                \includegraphics[width=\linewidth]{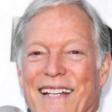}
                \caption{0\_5867244/3}
            \end{subfigure}
            \begin{subfigure}[b]{0.24\linewidth}
                \includegraphics[width=\linewidth]{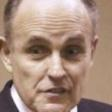}
                \caption{Rudolph\_Giuliani\_20}
            \end{subfigure}
            \begin{subfigure}[b]{0.24\linewidth}
                \includegraphics[width=\linewidth]{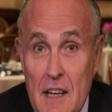}
                \caption{0\_5827623/79}
            \end{subfigure}       
        \end{subfigure}
        \begin{subfigure}[b]{1\linewidth}
            \begin{subfigure}[b]{0.24\linewidth}
                \includegraphics[width=\linewidth]{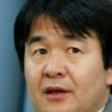}
                \caption{Heizo\_Takenaka\_7}
            \end{subfigure}
            \begin{subfigure}[b]{0.24\linewidth}
                \includegraphics[width=\linewidth]{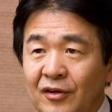}
                \caption{0\_5880926/6}
            \end{subfigure}
            \begin{subfigure}[b]{0.24\linewidth}
                \includegraphics[width=\linewidth]{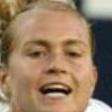}
                \caption{Elena\_Bovina\_1}
            \end{subfigure}
            \begin{subfigure}[b]{0.24\linewidth}
                \includegraphics[width=\linewidth]{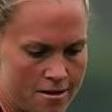}
                \caption{0\_5898207/98}
            \end{subfigure}
        \end{subfigure}
        \begin{subfigure}[b]{1\linewidth}
            \begin{subfigure}[b]{0.24\linewidth}
                \includegraphics[width=\linewidth]{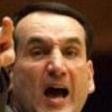}
                \caption{Mike\_Krzyzewski\_2}
            \end{subfigure}
            \begin{subfigure}[b]{0.24\linewidth}
                \includegraphics[width=\linewidth]{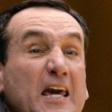}
                \caption{0\_5846710/46}
            \end{subfigure}
            \begin{subfigure}[b]{0.24\linewidth}
                \includegraphics[width=\linewidth]{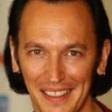}
                \caption{Steve\_Valentine\_1}
            \end{subfigure}
            \begin{subfigure}[b]{0.24\linewidth}
                \includegraphics[width=\linewidth]{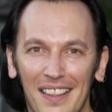}
                \caption{0\_5879521/72}
            \end{subfigure}
        \end{subfigure}
    \end{subfigure}
   \caption{Examples of the same identity occur in both LFW and MS1MV2. 
   }
\label{fig:same-identity-1}
\end{figure*}

\begin{figure*}[t]
    \centering
    \captionsetup[subfigure]{labelformat=empty}
    \begin{subfigure}[b]{0.9\linewidth}
        \begin{subfigure}[b]{1\linewidth}
            \begin{subfigure}[b]{0.24\linewidth}
                \includegraphics[width=\linewidth]{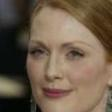}
                \caption{Julianne\_Moore\_15}
            \end{subfigure}
            \begin{subfigure}[b]{0.24\linewidth}
                \includegraphics[width=\linewidth]{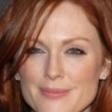}
                \caption{0\_5837950/82}
            \end{subfigure}
            \begin{subfigure}[b]{0.24\linewidth}
                \includegraphics[width=\linewidth]{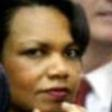}
                \caption{Condoleezza\_Rice\_5}
            \end{subfigure}
            \begin{subfigure}[b]{0.24\linewidth}
                \includegraphics[width=\linewidth]{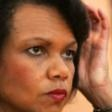}
                \caption{0\_5835176/91}
            \end{subfigure}
        \end{subfigure}
        \begin{subfigure}[b]{1\linewidth}
            \begin{subfigure}[b]{0.24\linewidth}
                \includegraphics[width=\linewidth]{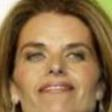}
                \caption{Maria\_Shriver\_2}
            \end{subfigure}
            \begin{subfigure}[b]{0.24\linewidth}
                \includegraphics[width=\linewidth]{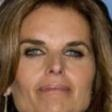}
                \caption{0\_5842997/68}
            \end{subfigure}
            \begin{subfigure}[b]{0.24\linewidth}
                \includegraphics[width=\linewidth]{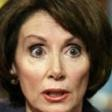}
                \caption{Nancy\_Pelosi\_9}
            \end{subfigure}
            \begin{subfigure}[b]{0.24\linewidth}
                \includegraphics[width=\linewidth]{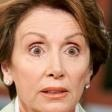}
                \caption{0\_5885609/106}
            \end{subfigure}
        \end{subfigure}

        \begin{subfigure}[b]{1\linewidth}
            \begin{subfigure}[b]{0.24\linewidth}
                \includegraphics[width=\linewidth]{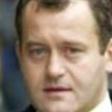}
                \caption{Paul\_Burrell\_10}
            \end{subfigure}
            \begin{subfigure}[b]{0.24\linewidth}
                \includegraphics[width=\linewidth]{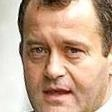}
                \caption{0\_5834783/33}
            \end{subfigure}
            \begin{subfigure}[b]{0.24\linewidth}
                \includegraphics[width=\linewidth]{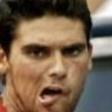}
                \caption{Mark\_Philippoussis\_2}
            \end{subfigure}
            \begin{subfigure}[b]{0.24\linewidth}
                \includegraphics[width=\linewidth]{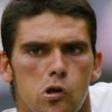}
                \caption{0\_5839025/21}
            \end{subfigure}       
        \end{subfigure}
        \begin{subfigure}[b]{1\linewidth}
            \begin{subfigure}[b]{0.24\linewidth}
                \includegraphics[width=\linewidth]{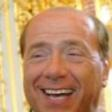}
                \caption{Silvio\_Berlusconi\_32}
            \end{subfigure}
            \begin{subfigure}[b]{0.24\linewidth}
                \includegraphics[width=\linewidth]{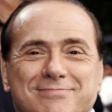}
                \caption{0\_5882840/33}
            \end{subfigure}
            \begin{subfigure}[b]{0.24\linewidth}
                \includegraphics[width=\linewidth]{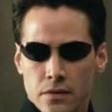}
                \caption{Keanu\_Reeves\_7}
            \end{subfigure}
            \begin{subfigure}[b]{0.24\linewidth}
                \includegraphics[width=\linewidth]{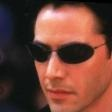}
                \caption{0\_5865903/110}
            \end{subfigure}
        \end{subfigure}
        \begin{subfigure}[b]{1\linewidth}
            \begin{subfigure}[b]{0.24\linewidth}
                \includegraphics[width=\linewidth]{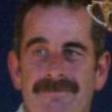}
                \caption{Sam\_Torrance\_3}
            \end{subfigure}
            \begin{subfigure}[b]{0.24\linewidth}
                \includegraphics[width=\linewidth]{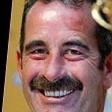}
                \caption{0\_5880918/14}
            \end{subfigure}
            \begin{subfigure}[b]{0.24\linewidth}
                \includegraphics[width=\linewidth]{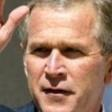}
                \caption{George\_W\_Bush\_150}
            \end{subfigure}
            \begin{subfigure}[b]{0.24\linewidth}
                \includegraphics[width=\linewidth]{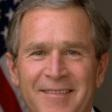}
                \caption{0\_5841527/34}
            \end{subfigure}
        \end{subfigure}
    \end{subfigure}
   \caption{Examples of the same identity occur in both LFW and MS1MV2. 
   }
\label{fig:same-identity-2}
\end{figure*}
