# Supplementary material for: Identity Overlap Between Face Recognition Train/Test Data: Causing Optimistic Bias in Accuracy Measurement
Source: arXiv:2405.09403 source file (2024-05-15)
Supplement: Supplementary file 2 [file cplfw-no-face.tex]

\begin{figure}[h]
    \centering
    \captionsetup[subfigure]{labelformat=empty}
    \begin{subfigure}[b]{1\linewidth}
        \begin{subfigure}[b]{1\linewidth}
            \begin{subfigure}[b]{0.19\linewidth}
                \includegraphics[width=\linewidth]{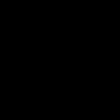}
            \end{subfigure}
            \begin{subfigure}[b]{0.19\linewidth}
                \includegraphics[width=\linewidth]{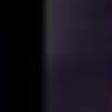}
            \end{subfigure}
            \begin{subfigure}[b]{0.19\linewidth}
                \includegraphics[width=\linewidth]{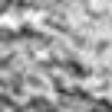}
            \end{subfigure}
            \begin{subfigure}[b]{0.19\linewidth}
                \includegraphics[width=\linewidth]{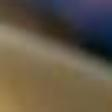}
            \end{subfigure}
            \begin{subfigure}[b]{0.19\linewidth}
                \includegraphics[width=\linewidth]{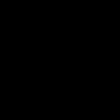}
            \end{subfigure}
        \end{subfigure}
        \begin{subfigure}[b]{1\linewidth}
            \begin{subfigure}[b]{0.19\linewidth}
                \includegraphics[width=\linewidth]{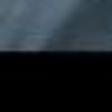}
            \end{subfigure}
            \begin{subfigure}[b]{0.19\linewidth}
                \includegraphics[width=\linewidth]{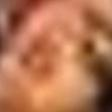}
            \end{subfigure}
            \begin{subfigure}[b]{0.19\linewidth}
                \includegraphics[width=\linewidth]{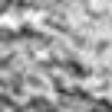}
            \end{subfigure}
            \begin{subfigure}[b]{0.19\linewidth}
                \includegraphics[width=\linewidth]{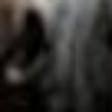}
            \end{subfigure}
            \begin{subfigure}[b]{0.19\linewidth}
                \includegraphics[width=\linewidth]{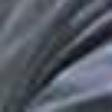}
            \end{subfigure}
        \end{subfigure}
        
    \end{subfigure}
   \caption{Examples of no-face images in the CPLFW .bin file.}
\label{fig:no-face}
\end{figure}
