# Supplementary material for: Identity Overlap Between Face Recognition Train/Test Data: Causing Optimistic Bias in Accuracy Measurement
Source: arXiv:2405.09403 source file (2024-05-15)
Supplement: Supplementary file 4 [file same_images.tex]

\begin{figure*}[t]
    \centering
    \captionsetup[subfigure]{labelformat=empty}
    \begin{subfigure}[b]{0.9\linewidth}
        \begin{subfigure}[b]{1\linewidth}
            \begin{subfigure}[b]{0.24\linewidth}
                \includegraphics[width=\linewidth]{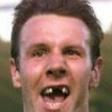}
                \caption{Craig\_Burley\_1}
            \end{subfigure}
            \begin{subfigure}[b]{0.24\linewidth}
                \includegraphics[width=\linewidth]{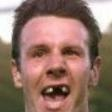}
                \caption{0\_5890009/57}
            \end{subfigure}
            \begin{subfigure}[b]{0.24\linewidth}
                \includegraphics[width=\linewidth]{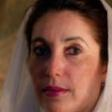}
                \caption{Benazir\_Bhutto\_2}
            \end{subfigure}
            \begin{subfigure}[b]{0.24\linewidth}
                \includegraphics[width=\linewidth]{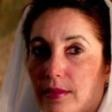}
                \caption{0\_5836537/26}
            \end{subfigure}
        \end{subfigure}
        \begin{subfigure}[b]{1\linewidth}
            \begin{subfigure}[b]{0.24\linewidth}
                \includegraphics[width=\linewidth]{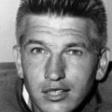}
                \caption{Johnny\_Unitas\_2}
            \end{subfigure}
            \begin{subfigure}[b]{0.24\linewidth}
                \includegraphics[width=\linewidth]{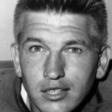}
                \caption{0\_5856661/23}
            \end{subfigure}
            \begin{subfigure}[b]{0.24\linewidth}
                \includegraphics[width=\linewidth]{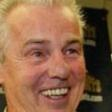}
                \caption{Doug\_Moe\_1}
            \end{subfigure}
            \begin{subfigure}[b]{0.24\linewidth}
                \includegraphics[width=\linewidth]{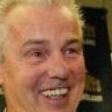}
                \caption{0\_5872926/6}
            \end{subfigure}
        \end{subfigure}

        \begin{subfigure}[b]{1\linewidth}
            \begin{subfigure}[b]{0.24\linewidth}
                \includegraphics[width=\linewidth]{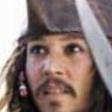}
                \caption{Johnny\_Depp\_1}
            \end{subfigure}
            \begin{subfigure}[b]{0.24\linewidth}
                \includegraphics[width=\linewidth]{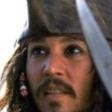}
                \caption{0\_5892154/67}
            \end{subfigure}
            \begin{subfigure}[b]{0.24\linewidth}
                \includegraphics[width=\linewidth]{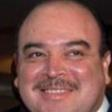}
                \caption{Cruz\_Bustamante\_4}
            \end{subfigure}
            \begin{subfigure}[b]{0.24\linewidth}
                \includegraphics[width=\linewidth]{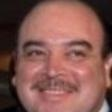}
                \caption{0\_5840766/21}
            \end{subfigure}       
        \end{subfigure}
        \begin{subfigure}[b]{1\linewidth}
            \begin{subfigure}[b]{0.24\linewidth}
                \includegraphics[width=\linewidth]{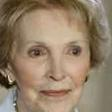}
                \caption{Nancy\_Reagan\_1}
            \end{subfigure}
            \begin{subfigure}[b]{0.24\linewidth}
                \includegraphics[width=\linewidth]{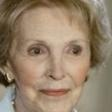}
                \caption{0\_5874109/26}
            \end{subfigure}
            \begin{subfigure}[b]{0.24\linewidth}
                \includegraphics[width=\linewidth]{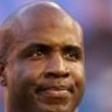}
                \caption{Barry\_Bonds\_1}
            \end{subfigure}
            \begin{subfigure}[b]{0.24\linewidth}
                \includegraphics[width=\linewidth]{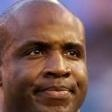}
                \caption{0\_5836919/19}
            \end{subfigure}
        \end{subfigure}
        \begin{subfigure}[b]{1\linewidth}
            \begin{subfigure}[b]{0.24\linewidth}
                \includegraphics[width=\linewidth]{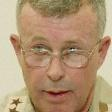}
                \caption{David\_McKiernan\_1}
            \end{subfigure}
            \begin{subfigure}[b]{0.24\linewidth}
                \includegraphics[width=\linewidth]{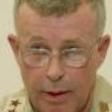}
                \caption{0\_5897287/3}
            \end{subfigure}
            \begin{subfigure}[b]{0.24\linewidth}
                \includegraphics[width=\linewidth]{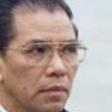}
                \caption{Nong\_Duc\_Manh\_1}
            \end{subfigure}
            \begin{subfigure}[b]{0.24\linewidth}
                \includegraphics[width=\linewidth]{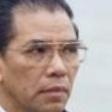}
                \caption{0\_5836715/40}
            \end{subfigure}
        \end{subfigure}
    \end{subfigure}
   \caption{Examples of the same images occur in both LFW and MS1MV2. 
   }
\label{fig:same-image-1}
\end{figure*}

\begin{figure*}[t]
    \centering
    \captionsetup[subfigure]{labelformat=empty}
    \begin{subfigure}[b]{0.9\linewidth}
        \begin{subfigure}[b]{1\linewidth}
            \begin{subfigure}[b]{0.24\linewidth}
                \includegraphics[width=\linewidth]{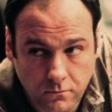}
                \caption{James\_Gandolfini\_2}
            \end{subfigure}
            \begin{subfigure}[b]{0.24\linewidth}
                \includegraphics[width=\linewidth]{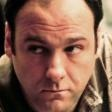}
                \caption{0\_5854640/22}
            \end{subfigure}
            \begin{subfigure}[b]{0.24\linewidth}
                \includegraphics[width=\linewidth]{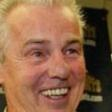}
                \caption{Doug\_Moe\_1}
            \end{subfigure}
            \begin{subfigure}[b]{0.24\linewidth}
                \includegraphics[width=\linewidth]{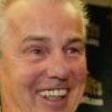}
                \caption{0\_5872926/0}
            \end{subfigure}
        \end{subfigure}
        \begin{subfigure}[b]{1\linewidth}
            \begin{subfigure}[b]{0.24\linewidth}
                \includegraphics[width=\linewidth]{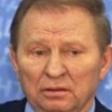}
                \caption{Leonid\_Kuchma\_1}
            \end{subfigure}
            \begin{subfigure}[b]{0.24\linewidth}
                \includegraphics[width=\linewidth]{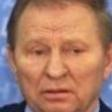}
                \caption{0\_5844623/57}
            \end{subfigure}
            \begin{subfigure}[b]{0.24\linewidth}
                \includegraphics[width=\linewidth]{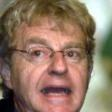}
                \caption{Jerry\_Springer\_1}
            \end{subfigure}
            \begin{subfigure}[b]{0.24\linewidth}
                \includegraphics[width=\linewidth]{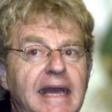}
                \caption{0\_5841902/102}
            \end{subfigure}
        \end{subfigure}

        \begin{subfigure}[b]{1\linewidth}
            \begin{subfigure}[b]{0.24\linewidth}
                \includegraphics[width=\linewidth]{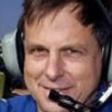}
                \caption{Ilan\_Ramon\_1}
            \end{subfigure}
            \begin{subfigure}[b]{0.24\linewidth}
                \includegraphics[width=\linewidth]{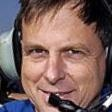}
                \caption{0\_5835892/65}
            \end{subfigure}
            \begin{subfigure}[b]{0.24\linewidth}
                \includegraphics[width=\linewidth]{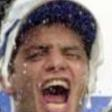}
                \caption{Alex\_Barros\_2}
            \end{subfigure}
            \begin{subfigure}[b]{0.24\linewidth}
                \includegraphics[width=\linewidth]{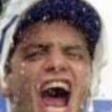}
                \caption{0\_5883749/5}
            \end{subfigure}       
        \end{subfigure}
        \begin{subfigure}[b]{1\linewidth}
            \begin{subfigure}[b]{0.24\linewidth}
                \includegraphics[width=\linewidth]{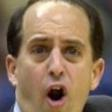}
                \caption{Jeff\_Van\_Gundy\_1}
            \end{subfigure}
            \begin{subfigure}[b]{0.24\linewidth}
                \includegraphics[width=\linewidth]{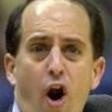}
                \caption{0\_5879676/6}
            \end{subfigure}
            \begin{subfigure}[b]{0.24\linewidth}
                \includegraphics[width=\linewidth]{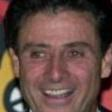}
                \caption{Rick\_Pitino\_3}
            \end{subfigure}
            \begin{subfigure}[b]{0.24\linewidth}
                \includegraphics[width=\linewidth]{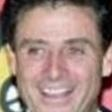}
                \caption{0\_5859710/8}
            \end{subfigure}
        \end{subfigure}
        \begin{subfigure}[b]{1\linewidth}
            \begin{subfigure}[b]{0.24\linewidth}
                \includegraphics[width=\linewidth]{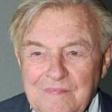}
                \caption{Teddy\_Kollek\_1}
            \end{subfigure}
            \begin{subfigure}[b]{0.24\linewidth}
                \includegraphics[width=\linewidth]{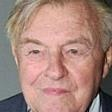}
                \caption{0\_5860410/31}
            \end{subfigure}
            \begin{subfigure}[b]{0.24\linewidth}
                \includegraphics[width=\linewidth]{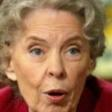}
                \caption{Jeane\_Kirkpatrick\_1}
            \end{subfigure}
            \begin{subfigure}[b]{0.24\linewidth}
                \includegraphics[width=\linewidth]{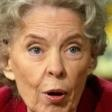}
                \caption{0\_5837214/13}
            \end{subfigure}
        \end{subfigure}
    \end{subfigure}
   \caption{Examples of the same image occur in both LFW and MS1MV2. 
   }
\label{fig:same-image-2}
\end{figure*}
